# Supplementary material for: Automated Neuron Shape Analysis from Electron Microscopy
Source: arXiv:2006.00100 source file (2020-05-29)
Supplement: Supplementary file 1 [file supplementary_material.tex]

\begin{algorithm}[H]
\SetCustomAlgoRuledWidth{0.53\textwidth} 
\caption{$ ShapeExtraction $}\label{alg:ext}
\begin{algorithmic}[1]

\Procedure{ShapeExtract}{$M$, $S_M$} 

\State $K \gets MeshSkeletonize(M)$ 

\State \For {$ s \in S_{M}$}
{$M^{s} \gets $ local mesh around $s$

$\mathcal{M}^{s} = \{ M^s_0 ... \} \gets Seg(M^{s})$

$x^{s} \gets$ closest point on $M^{s}$ %to $s$

$p \gets shortestPath(K,x^s)$ 

$\mathcal{M}^{s}_{p} = Prune(\mathcal{M}^{s}, p ) $

 Set $\overline M^s \gets \cup \mathcal{M}^{s}_{p} $

SHAPES $+= \overline M^s$}

\EndFor
\Return SHAPES

\EndProcedure
\end{algorithmic}
\end{algorithm}
